# Supplementary material for: Evidence for room temperature superconductivity associated with a first-order phase transition
Source: arXiv:2306.13172 ancillary file (2026-05-03)
Supplement: Supplementary file 1 [file SupplementaryMaterial-v3.pdf]

## **Supplementary material for**

### **Sayonara BCS: Realization of Room Temperature Superconductivity as a result of a First Order Phase Transition**

N. Zen

*National Institute of Advanced Industrial Science and Technology,  
Tsukuba Central 2-10, Ibaraki 305-8568, Japan*

---

In this Supplementary material,  $R$ – $T$  results for 18 different samples are shown. Among them, 5 samples were taken from a microfabricated wafer numbered I, and 13 samples were taken from another wafer numbered II. All the samples have a rectangular shape, the same as the one used in the main article. Among the examined 18 samples, 7 samples have exhibited zero resistance at room temperature.  $R$ – $T$  results for the rest which did not show zero resistance are also shown. Those results include some points that are not well understood at this time and may not be suitable for publication as a supplementary material for a paper. However, I decided to publish them in the hope that they may be of some use to third parties in their follow-up studies of this research. All figures in this Supplementary material are generated from raw data, and all the raw data are also available at a public repository, so please refer to them along with this Supplementary material.

---

[WAFER I, the sample fabrication completed on September 2021]

Figures S1 and S2 are  $R$ - $T$  results for the rectangular samples taken from the wafer I.

For each measurement, two or three sample chips were installed in the PPMS, and their  $R$ - $T$  characteristics were measured under the same condition.

(The PPMS can measure the maximum of three samples at the same time.)

- All samples have the  $d$  of 150 nm and  $a$  of 20  $\mu\text{m}$ , the same as those used for the main article.
- All measurements were performed under zero magnetic field.
- All measurements were performed using the two-probe method.

Only the first and the last  $R$ - $T$  cycles are shown.

All raw data including results for the rest of  $R$ - $T$  cycles have been uploaded at a public repository [54].

Figure S1 (a) and (b) show zero resistance at room temperature. The two-probe zero resistance indicates that it is not related to the voltage vanishing across the voltage electrodes, which is specific to four-probe measurements [13]. Figure S1(a) is the one that used in the main article. Samples for Fig. S1(b) and (c) have the same  $d$  and  $a$  as those of the sample used for Fig. S1(a) but have a larger area,  $4.0 \times 4.0 \text{ mm}^2$ . That is, the zero-resistance state presented in this study is attainable regardless of the sample size. Although Fig. S1(c) does not show anomalies, its  $R$ - $T$  curves being typical for normal Nb indicate that the thermometer of PPMS was working properly during the whole  $R$ - $T$  cycles.

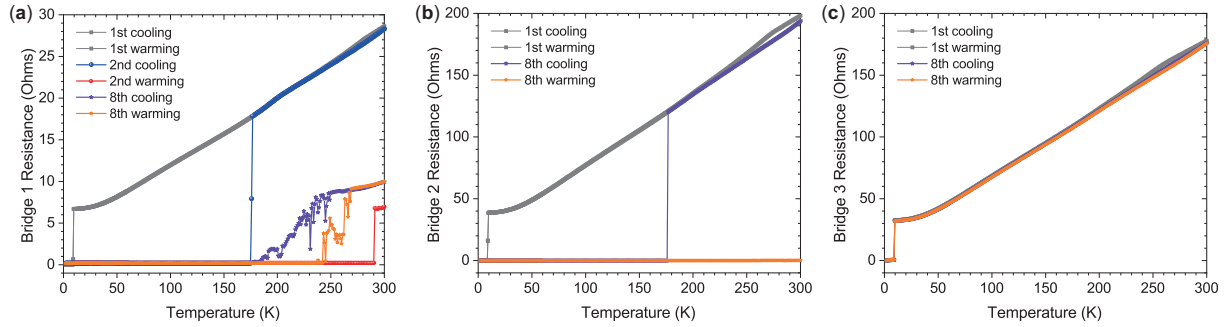

**Figure S1.** Measurement started on 21 September 2021. (a) Sample area is  $0.3 \times 0.5 \text{ mm}^2$ . (b) Sample area is  $4.0 \times 4.0 \text{ mm}^2$ . (c) Sample area is  $4.0 \times 4.0 \text{ mm}^2$ .

Neither Fig. S2(a) nor (b) shows zero resistance at high temperatures at least in the tested eight  $R$ - $T$  cycles. The resistance in (a) during the fourth cooling process gradually increased around 175 K.

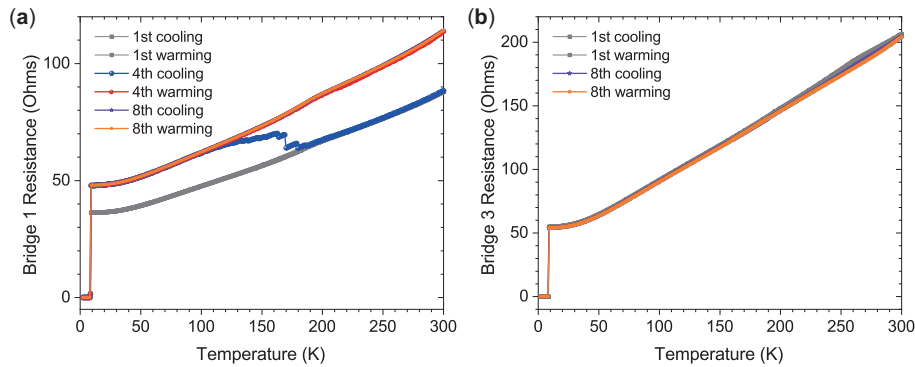

**Figure S2.** Measurement started on 29 October 2021. Bridge 2 is blank. Both samples for (a) and (b) have the area of  $4.0 \times 4.0 \text{ mm}^2$ .

[WAFER II, the sample fabrication completed on November 2018]

Figures S3–S8 are  $R$ – $T$  results for the rectangular samples taken from the wafer II.

For each measurement, two or three sample chips were installed in the PPMS at the same time, and their  $R$ – $T$  characteristics were measured under the same condition.

Only the first and the last  $R$ – $T$  cycles are shown.

All raw data including results for the rest of  $R$ – $T$  cycles have been uploaded at [54].

- All samples have the  $d$  of 150 nm and the area of  $0.3 \times 0.5 \text{ mm}^2$ .
- Except Fig. S3(b), all samples have the  $a$  of 20  $\mu\text{m}$ , the same as that used for the main article.
- Except Fig. S7, all measurements were performed under zero magnetic field.
- Except Fig. S8, all measurements were performed using the four-probe method.

Figure S3(a) shows zero resistance at room temperature; as the temperature was increased in the 25th “warming” process, the resistance dropped to zero at 50–60 K, and the zero-resistance state was retained at higher temperatures. The significance of “warming” is discussed in the main article associated with the universal GL theory for a first order phase transition. The sample for Fig. S3(b) exhibited anomalous rises and falls in resistance during temperature cycles at 35 K, 50 K, 80 K and around 200 K. The rise in resistance, the direction of which is opposed to superconductivity, indicates the onset of electron localization. In the metallic, oxygen-deficient system, the line between superconductivity and electron localization is thin, as in the Ba-La-Cu-O system reported in 1986 [10].

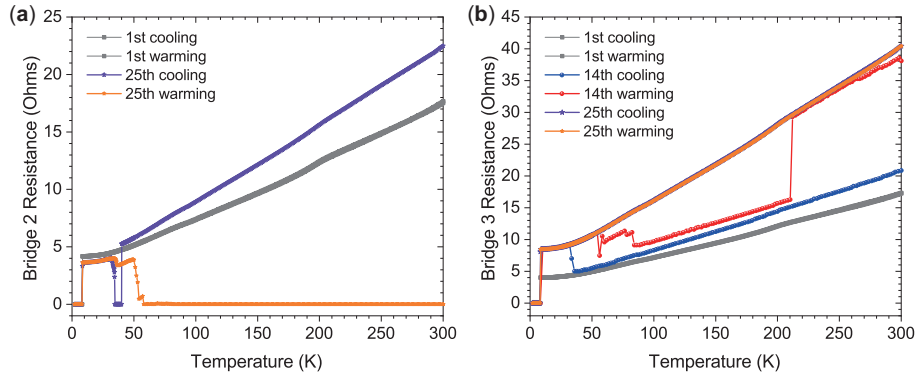

**Figure S3.** Measurement started on 16 November 2018. (a) Lattice constant  $a$  is 20  $\mu\text{m}$ . (b) Lattice constant  $a$  is 40  $\mu\text{m}$ .

Neither Fig. S4(a) nor (b) shows zero resistance at high temperatures during the tested 22  $R$ – $T$  cycles.

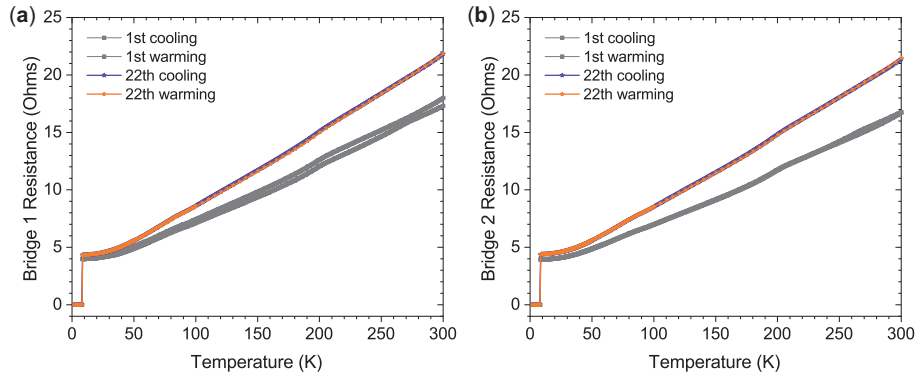

**Figure S4.** Measurement started on 28 December 2018.

Both Fig. S5(a) and (b) show a resistance drop at 100 K in the 12th “warming” process, but only (a) shows a clear zero resistance surviving at room temperature. The sample for Fig. S5(c) exhibited a rise and fall in resistance at 175 K and around 230 K, indicating electron localization.

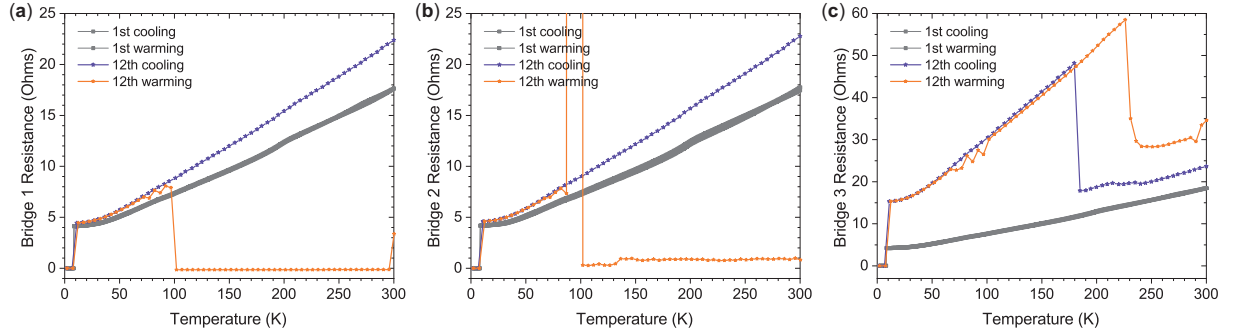

**Figure S5.** Measurement started on 10 December 2018.

Figure S6(a) shows zero resistance at room temperature; as the temperature was increased in the 21th “warming” process, the resistance dropped to zero at 35 K, and the zero-resistance state was retained at higher temperatures. However, it slightly increased to a finite value at a temperature above 280 K.

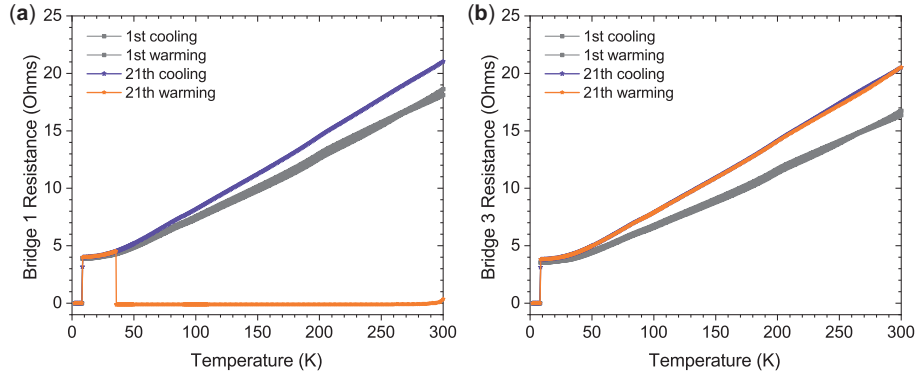

**Figure S6.** Measurement started on 08 February 2019.

Resistance of the sample for Fig. S7(a) dropped to zero at 50–60 K in the 17th “warming” process, and the zero resistance was retained at room temperature. Both Fig. S7(a) and (b) show very complicated  $R$ – $T$  curves, which are seemingly attributed to an applied magnetic field during the  $R$ – $T$  cycles. Although neither their details nor the observed negative resistance are well understood yet, the digitized  $R$ – $T$  behaviors, clearly seen especially for Fig. S7(b), might be an indication of resistive vortex motion taking place in the holey sample. The anomalous rises and falls in resistance occurred at 35 K, 50–60 K and around 100 K.

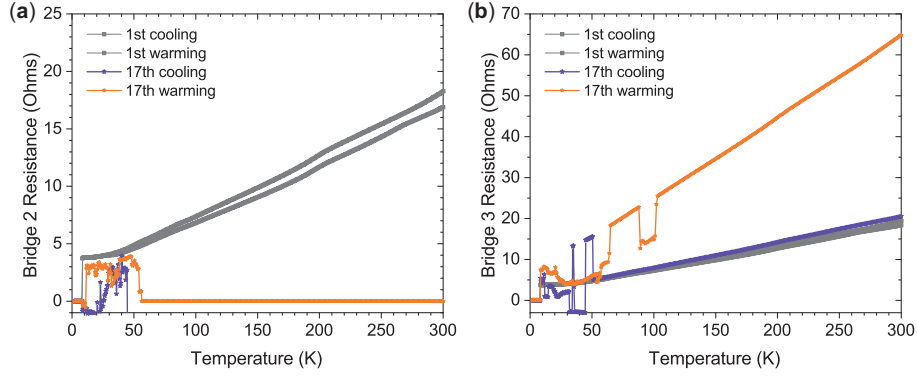

**Figure S7.** Measurement started on 26 April 2019. The measurement was performed under perpendicular magnetic field. For the 1st to 6th cycle, the magnitude was 10 Oe. For the 7th to 17th cycle, the magnitude was changed to 20 Oe.

Resistance of the sample for Fig. S8(b) dropped to zero at 50–60 K in the 18th “warming” process. But unfortunately, the resistance at temperatures higher than 80 K could not be measured because of disconnection of aluminum bonded wires. This proves that if electrical issues such as contact breaking occur during the  $R$ – $T$  measurement, the PPMS displays an error code and stops recording the resistance. That is to say, all the seven zero resistances reported above are not due to technical problems. There must be a new physics or superconductivity as the solid foundation for the zero resistance.

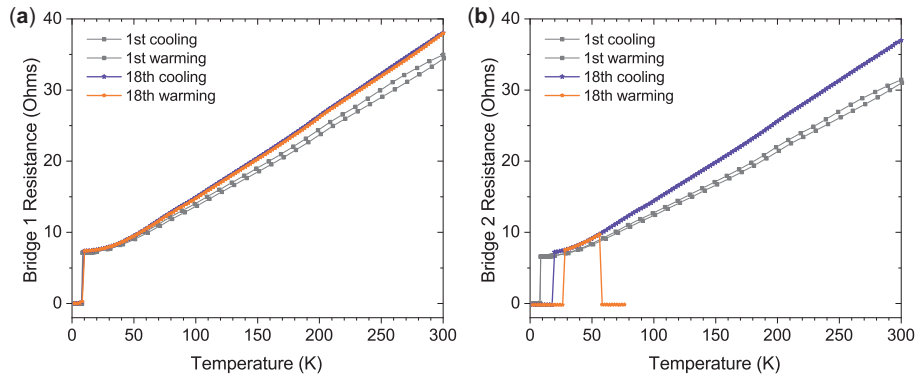

**Figure S8.** Measurement started on 26 June 2020. Both (a) and (b) were obtained using the two-probe method.

## Summary regarding Figs. S1–S8

To date, 18 PnM samples in a rectangular shape were examined, and 7 samples exhibited zero resistance at room temperature. So the yield rate is 39%, not high, but not low.

There are several common features in the  $R$ – $T$  measurements that yielded zero resistance, namely:

- (1) The  $R$ – $T$  cycles were repeatedly performed with the slow temperature sweep rate.  
(A typical  $R$ – $T$  recipe is shown in Table I in the main article.)
- (2) The zero resistance state persisted to higher temperatures *always* in a *warming* process.
- (3) The temperature at which a resistance dropped to zero has a typical value: 35K, 50K, 100K, 175K.
- (4) Whether the two- or four-probe measurement is not important.
- (5) A larger sample size is also worth trying.  
(The maximum size of the sample showing zero resistance is so far  $4.0 \times 4.0 \text{ mm}^2$ .)

The necessity of (1) might be related to oxygenation and its ordering in the bridge-like parts composing the holey sample, as discussed in the section III-E of the main article.

The reason for (2) is explained in the section III-A, based on the Ginzburg-Landau theory for a first order phase transition. According to Halperin, Lubensky, and Ma, any superconducting transition must *always* be first order [26]. Dynamics of the first order phase transition is discussed on the basis of the theory of hole superconductivity proposed by Hirsch [14].

Regarding (3), these temperatures are not only typical as a  $T_c$  indicating zero resistance. They are also typical as the temperature at which the samples that did not eventually achieve zero resistance show a rise and fall in resistance. For example, a rise in resistance occurs at 175 K in Fig. S2(a); rises and falls in resistance occur at 35 K, 50 K, 80 K and around 200 K in Fig. S3(b); a fall in resistance occurs at 100 K in Fig. S5(b); a rise and fall occur at 175 K and around 230 K in Fig. S5(c); rises and falls occur at 35 K, 50 K and around 100 K in Fig. S7(b). This fact that the onset of zero resistance and the rises and falls in resistance occur at the same temperature range rather supports our assumption of percolative superconductivity in the holey sample discussed in the section III-A. By taking into account the heterogeneity of oxygen concentrations in bridge-like parts as indicated by the SEM-EDX image in Fig. 3, it is possible that the sample under study is composed of a mixture of superconducting and nonsuperconducting paths. For the sample with such a percolative superconductivity, an obvious zero resistance is achieved only when the percolation seeps through the holey sheet to the electrodes for measuring resistance. If this does not happen, the resistance of such a sample that does not have a full superconducting path between electrodes would just repeatedly rise and fall during temperature cycles. The reason why those temperatures cannot be answered now, because we don't even know yet why a monumental superconductor YBCO shows the  $T_c$  of 90 K. In addition, the rise in resistance may also be attributed to electron localization. In a metallic, oxygen-deficient system such as the one in this study, it is not easy to predict whether electrons will become superconducting or localized. This was also the focus of debate when the Ba-La-Cu-O system—the herald of cuprate high- $T_c$  superconductivity era—was first reported to the public [10]. Just as bulk superconductivity of cuprates was later improved, that of the system presented in this study will also be improved in the future.

Regarding (4), three of the seven samples showing zero resistance were measured by the two-probe method. This fact dispels a mundane speculation that the zero resistance is due to a vanishing four-probe resistance in non-superconducting systems [13]. I believe there is no other explanation than attributing the observed zero resistance to superconductivity.

Again, the PPMS displays an error code and stops recording resistance data if electrical issues such as contact breaking or wire disconnection occur during the  $R$ - $T$  measurement. In other words, all the zero resistance, which have been clearly shown in this study and whose correctness and accuracy can be confirmed in the raw data [54], are not due to technical problems or measurement errors. There must be the solid foundation for the zero resistance state.

## References

- [10] J. G. Bednorz, K. A. Müller, Possible high  $T_c$  superconductivity in the Ba-La-Cu-O system, *Z. Phys. B* **64** (1986) 189–193, <https://doi.org/10.1007/BF01303701>.
- [13] S. Urazhdin, Comment on arXiv:1807.08572, “Coexistence of Diamagnetism and Vanishingly Small Electrical Resistance at Ambient Temperature and Pressure in Nanostructures”, arXiv:1906.05742v1 (Submission: 13 June 2019), <https://arxiv.org/abs/1906.05742>.
- [14] J. E. Hirsch, Magnetic flux expulsion in a superconducting wire, *Phys. Lett. A* **413** (2021) 127592, <https://doi.org/10.1016/j.physleta.2021.127592>.
- [26] B. I. Halperin, T. C. Lubensky, S.-K. Ma, First-Order Phase Transitions in Superconductors and Smectic-A Liquid Crystals, *Phys. Rev. Lett.* **32** (1974) 292–295, <https://doi.org/10.1103/PhysRevLett.32.292>.
- [54] N. Zen, Raw data for High temperature superconductivity arising in a metal sheet full of holes, *Zenodo* (Publication: 15 July 2022) v5, <https://doi.org/10.5281/zenodo.5885550>.
